# Supplementary material for: Electrotactile Feedback For Enhancing Contact Information in Virtual Reality
Source: arXiv:2102.00259 source file (2021-09-21)
Supplement: Supplementary file 1 [file SupplementaryMaterial__1_.pdf]

# Evaluating electrotactile feedback for contact rendering of virtual surfaces: supplemental document

**Maximum Index Interpenetration:** The descriptive data are displayed in Table S1. The outcomes of the ANOVA postulated that all the effects were statistically significant at the .05 significance level. The main effect for the type of feedback yielded a main effect of $F(1.88, 37.52) = 28.36, p < .001$ suggesting a significant difference between the diverse feedback types. Also, an $\rightarrow^2 = 0.56, 95\%\ CI[0.38, 0.68]$ was calculated, indicating a very large effect size of the type of feedback on maximum interpenetration. Similarly, the main effect for the experiment's part produced a main effect of $F(1, 20) = 29.43, p < .001$ indicating a significant difference between the two parts of the experiment. An $\rightarrow^2 = 0.56, 95\%\ CI[0.24, 0.74]$ was yielded equally suggesting a very large effect size of the part of experiment on maximum interpenetration. Lastly, the interaction effect between the type of feedback and the part of experiment produced an effect of $F(2.06, 41.24) = 5.16, p = .009$ postulating a significant difference amongst the diverse pairs derived from the parts of the experiment and the types of feedback. An $\rightarrow^2 = 0.16, 95\%\ CI - 0.02, 0.32]$ was yielded equally indicating a large effect size on maximum interpenetration by the interaction between the parts of the experiment and the types of feedback.

The post-hoc pairwise comparisons can be seen in Figure S1. In the $1^{st}$ part, the visual $g = 0.99, p < .001$ and combined feedback $g = 1.17, p < .001$ were significantly better than the non-feedback condition, with a large effect in both comparisons. Also, the visual $g = 0.59, p = .010$ and combined feedback $g = 0.73, p = .002$ were significantly better than the electrotactile condition, with a moderate effect size. In the $2^{nd}$ part, the visual $g = 1.26, p < .001$, combined $g = 1.79, p < .001$, and electrotactile feedback $g = 1.12, p < .001$, were substantially better than the non-feedback condition, with a very large effect in every comparison. No further significant differences were detected in both parts. Moreover, the electrotactile $g = 0.82, p < .001$ and combined feedback $g = 0.39, p = .004$ were significantly better in the $2^{nd}$ part compared to the $1^{st}$ part, with a large and a moderate effect respectively, while the equivalent comparisons for the non-feedback and visual feedback were not significant. Importantly, only the size of change for electrotactile feedback was substantially greater than the size of change for non-feedback $g = 0.62, p = .007$ and visual feedback $g = 0.60, p = .011$, with a moderate effect size in both comparisons.

**Table S1.** Maximum Interpenetration per Feedback and/or Part.

| | n | Mean (SD) | Range | SE |
|---|---|---|---|---|
| No Feedback | 42 | 1.72 (0.55) | 0.72 - 3.09 | 0.09 |
| Electrotactile Feedback | 42 | 1.36 (0.60) | 0.48 - 2.73 | 0.09 |
| Visual Feedback | 42 | 1.17 (0.54) | 0.54 - 3.07 | 0.08 |
| Combined Feedback | 42 | 1.04 (0.42) | 0.44 - 2.38 | 0.07 |
| Part 1 | 84 | 1.46 (0.63) | 0.47 - 3.09 | 0.07 |
| Part 2 | 84 | 1.18 (0.51) | 0.44 - 2.65 | 0.06 |
| No Feedback-Part 1 | 21 | 1.84 (0.66) | 0.75 - 3.09 | 0.14 |
| No Feedback-Part 2 | 21 | 1.59 (0.41) | 0.72 - 2.54 | 0.09 |
| Electrotactile Feedback-Part 1 | 21 | 1.58 (0.58) | 0.55 - 2.73 | 0.13 |
| Electrotactile Feedback-Part 2 | 21 | 1.13 (0.53) | 0.48 - 2.65 | 0.12 |
| Visual Feedback-Part 1 | 21 | 1.25 (0.62) | 0.58 - 3.07 | 0.13 |
| Visual Feedback-Part 2 | 21 | 1.08 (0.45) | 0.54 - 2.37 | 0.10 |
| Combined Feedback-Part 1 | 21 | 1.16 (0.44) | 0.47 - 2.38 | 0.10 |
| Combined Feedback-Part 2 | 21 | 0.92 (0.38) | 0.44 - 2.20 | 0.08 |

*The maximum interpenetration is displayed in centimetres;*

*SD = Standard Deviation; SE = Standard Error*

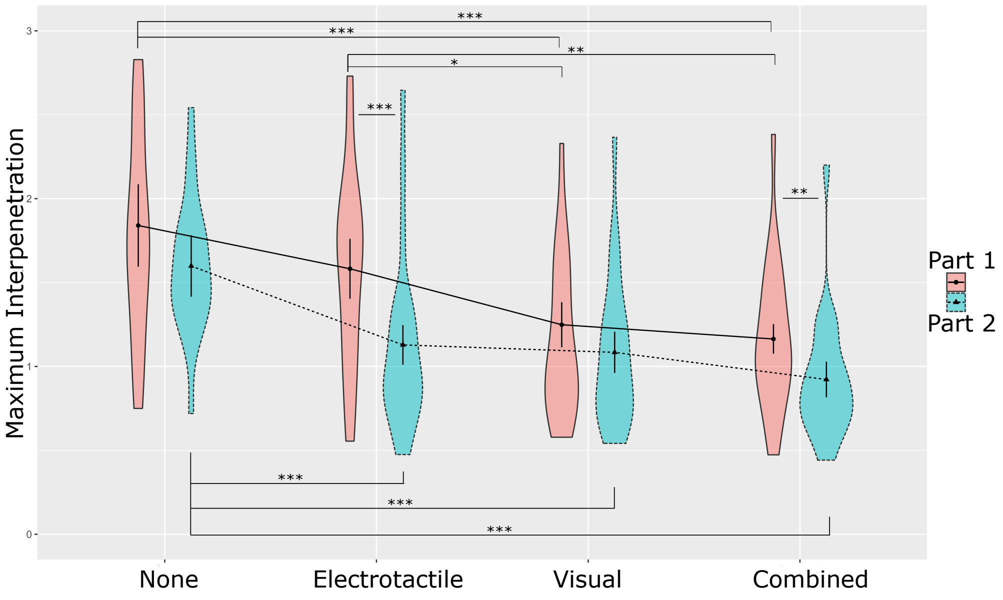


**Fig. S1.** Maximum Interpenetration Comparisons per Type of Feedback and Part of the Experiment

**Table S2.** Average Interpenetration per Feedback and/or Part.

| | n | Mean (SD) | Range | SE |
|---|---|---|---|---|
| No Feedback | 42 | 1.23 (0.40) | 0.53 - 2.14 | 0.06 |
| Electrotactile Feedback | 42 | 0.99 (0.47) | 0.35 - 2.23 | 0.07 |
| Visual Feedback | 42 | 0.87 (0.43) | 0.39 - 2.33 | 0.07 |
| Combined Feedback | 42 | 0.76 (0.34) | 0.31 - 1.75 | 0.05 |
| Part 1 | 84 | 1.08 (0.48) | 0.37 - 2.33 | 0.05 |
| Part 2 | 84 | 0.85 (0.38) | 0.31 - 2.05 | 0.04 |
| No Feedback-Part 1 | 21 | 1.32 (0.45) | 0.61 - 1.53 | 0.10 |
| No Feedback-Part 2 | 21 | 1.15 (0.33) | 0.53 - 2.05 | 0.07 |
| Electrotactile Feedback-Part 1 | 21 | 1.18 (0.48) | 0.42 - 2.23 | 0.11 |
| Electrotactile Feedback-Part 2 | 21 | 0.81 (0.37) | 0.35 - 1.84 | 0.08 |
| Visual Feedback-Part 1 | 21 | 0.94 (0.50) | 0.42- 2.33 | 0.11 |
| Visual Feedback-Part 2 | 21 | 0.80 (0.35) | 0.39 - 1.67 | 0.08 |
| Combined Feedback-Part 1 | 21 | 0.87 (0.35) | 0.37 - 1.75 | 0.08 |
| Combined Feedback-Part 2 | 21 | 0.66 (0.31) | 0.31 - 1.69 | 0.07 |

*The average interpenetration is displayed in centimetres;*

*SD = Standard Deviation; SE = Standard Error*

**Table S3.** Precision per Feedback and/or Part.

| | n | Mean (SD) | Range | SE |
|---|---|---|---|---|
| No Feedback | 42 | 0.23 (0.13) | 0.06 - 0.56 | 0.02 |
| Electrotactile Feedback | 42 | 0.17 (0.10) | 0.05 - 0.39 | 0.02 |
| Visual Feedback | 42 | 0.13 (0.08) | 0.05 - 0.45 | 0.01 |
| Combined Feedback | 42 | 0.12 (0.06) | 0.04 - 0.29 | 0.01 |
| Part 1 | 84 | 0.18 (0.11) | 0.04 - 0.56 | 0.01 |
| Part 2 | 84 | 0.15 (0.09) | 0.05 - 0.43 | 0.01 |
| No Feedback-Part 1 | 21 | 0.25 (0.14) | 0.06 - 0.56 | 0.03 |
| No Feedback-Part 2 | 21 | 0.22 (0.08) | 0.08 - 0.43 | 0.02 |
| Electrotactile Feedback-Part 1 | 21 | 0.20 (0.10) | 0.07 - 0.38 | 0.02 |
| Electrotactile Feedback-Part 2 | 21 | 0.14 (0.09) | 0.05 - 0.39 | 0.02 |
| Visual Feedback-Part 1 | 21 | 0.13 (0.09) | 0.05 - 0.45 | 0.02 |
| Visual Feedback-Part 2 | 21 | 0.13 (0.07) | 0.06 - 0.37 | 0.02 |
| Combined Feedback-Part 1 | 21 | 0.13 (0.06) | 0.04 - 0.29 | 0.01 |
| Combined Feedback-Part 2 | 21 | 0.11 (0.06) | 0.05 - 0.27 | 0.01 |

*The precision (finger's oscillations) is displayed in centimetres;*

*SD = Standard Deviation; SE = Standard Error*

**Table S4.** Intensity Values per Calibration Phase.

| | n | Mean (SD) | Range | SE |
|---|---|---|---|---|
| Initial - Sensation Threshold | 21 | 1.65 (0.91) | 0.60 - 4.10 | 0.20 |
| Middle - Sensation Threshold | 21 | 2.21 (1.12) | 0.90 - 5.30 | 0.24 |
| Final - Sensation Threshold | 21 | 2.21 (1.42) | 0.60 - 6.60 | 0.31 |
| Initial - Pain Threshold | 21 | 3.10 (1.66) | 1.20 - 7.60 | 0.36 |
| Middle - Pain Threshold | 21 | 4.26 (2.26) | 1.50 - 9.00 | 0.49 |
| Final - Pain Threshold | 21 | 4.09 (2.08) | 1.60 - 9.00 | 0.45 |
| Initial - Actual Value | 21 | 2.51 (1.35) | 1.00 - 6.20 | 0.29 |
| Middle - Actual Value | 21 | 3.43 (1.76) | 1.30 - 7.50 | 0.39 |
| Final - Actual Value | 21 | 3.34 (1.78) | 1.20 - 8.00 | 0.39 |

*The intensity values are displayed in milliamperes;*

*SD = Standard Deviation; SE = Standard Error*

## Post-Experience Questionnaire

### Functional questions

Regarding the visual feedback (for interpenetration), how useful it was helping you to complete the task accurately and fast?

1 Highly unhelpful
2 Very unhelpful
3 Unhelpful
4 Moderate
5 Useful
6 Very useful
7 Highly useful

Regarding the electrotactile feedback (for interpenetration), how useful it was helping you to complete the task accurately and fast?

1 Highly unhelpful
2 Very unhelpful
3 Unhelpful
4 Moderate
5 Useful
6 Very useful
7 Highly useful

In the condition with visual and tactile feedback, did you rely more on:

1 Fully on visual
2 Much more on visual
3 More on visual
4 Both
5 More on tactile
6 Much more on tactile
7 Fully on tactile

### Perception related questions

How much the elicited sensation by the tactile feedback resembles touching a real surface?

1 Extremely different
2 Very different
3 Different
4 Moderate
5 Similar
6 Very similar
7 Extremely similar

How much the elicited sensation by the visual feedback resembles touching a real surface?

1 Extremely different
2 Very different
3 Different
4 Moderate
5 Similar
6 Very similar
7 Extremely similar

How much the elicited sensation by the combined feedback resembles touching a real surface?

1 Extremely different
2 Very different
3 Different
4 Moderate
5 Similar
6 Very similar
7 Extremely similar

### Acceptability questions

How do you considered the sensation elicited by the electrotactile feedback

1 Extremely annoying
2 Very annoying
3 Annoying
4 Moderate
5 Pleasant
6 Very pleasant
7 Extremely pleasant

With the electrotactile feedback did you feel changes in the strength of the sensation while pressing down the surface?

1 Not at all
2 Very rarely
3 Rarely
4 Sometimes
5 Often
6 Very often
7 All the time

Regarding the motion of your finger and how you interacted with the object, was the electrotactile feedback coherent with your interaction?

1 Completely dissociated
2 Very dissociated
3 Dissociated
4 Moderate
5 Coherent
6 Very coherent
7 Completely coherent

Regarding the motion of your finger and how you interacted with the object, was the visual feedback coherent with your interaction?

1 Completely dissociated
2 Very dissociated
3 Dissociated
4 Moderate
5 Coherent
6 Very coherent
7 Completely coherent

Did you feel that visual and tactile feedback were synchronized?

1 Not at all
2 Very rarely
3 Rarely
4 Sometimes
5 Often
6 Very often
7 All the time

How enjoyable was the experience? (justify your answer)

1 Extremely annoying
2 Very annoying
3 Annoying
4 Moderate
5 Pleasant
6 Very pleasant
7 Extremely pleasant

How would you describe the sensation elicited by the electrotactile feedback? (open question)

**Fig. S2.** Post-exposure Questionnaire
